# Supplementary material for: ALANNO: An Active Learning Annotation System for Mortals
Source: arXiv:2211.06224 source file (2023-02-21)
Supplement: Supplementary file 1 [file appendix.tex]

\clearpage
\appendix

\section{}
\label{sec:A}
